# Supplementary material for: Dual-path Adaptation from Image to Video Transformers
Source: arXiv:2303.09857 source file (2023-03-17)
Supplement: Supplementary file 1 [file tab_imple.tex]

\begin{table*}[hbt!]
    \centering
    \small
    \setlength{\tabcolsep}{12pt}
    % \resizebox{0.95\linewidth}{!}{
        \begin{tabular}{l c c c c }
        \toprule
        Components &   K400~\cite{k400}    &  SSv2~\cite{ssv2}   & HMDB51~\cite{hmdb51}      & Diving-48~\cite{diving}  \\ 
        \midrule        
        \multicolumn{5}{l}{\hspace{-5pt}\textit{\textbf{Adapter}}} \\
        % AIM~\cite{aim} w/ ViT-B/16           &    CLIP   &   97M     &  11M  &    2428      &  84.7  & 96.7    &   32$\times$3$\times$1   \\
        % AIM~\cite{aim} w/  ViT-B/16           &    CLIP   &   97M     &  11M  &    1214      &  84.5  & 96.6    &   16$\times$3$\times$1   \\ 
        \# Adapters per block        &  4 (2 SP, 2 TP)  &  5 (2 SP, 3 TP)  &  4 (2 SP, 2 TP)  &  4 (2 SP, 2 TP)   \\
        Adapter bottleneck width        &  128  &  128  &  128  &  128  \\ \midrule
        \multicolumn{5}{l}{\hspace{-5pt}\textit{\textbf{Optimizer (AdamW~\cite{adamw}, Cosine scheduler~\cite{cosine-sched})}}} \\
        % Optimizer        &  \multicolumn{4}{c}{AdamW~\cite{adamw}, Cosine scheduler~\cite{cosine-sched}}  \\
        Learning rate        &  3e-4    &   5e-4    &   1e-4    &   3e-4  \\
        Weight Decay        &  5e-2    &   5e-2    &   2e-2    &   3e-2  \\
        Batch size        &  64    &   128  &   128 &   128  \\
        \midrule
        \multicolumn{5}{l}{\hspace{-5pt}\textit{\textbf{Data configuration}}} \\
        Training crop size        &  224    &   224     &   224     &      224  \\
        Frame sampling rate ($T_S$)        &  16 for $T_S=8$    &   16 for $T_S=8$  &   16 for $T_S=8$  &   16 for $T_S=8$  \\
        Frame sampling rate ($T_G$)        &  \makecell{8 for $T_G=1$ \\ 4 for $T_G=2$ \\ 2 for $T_G=3$}  & Dynamic sampling & \makecell{8 for $T_G=1$ \\ 4 for $T_G=2$ \\ 2 for $T_G=3$}  & \makecell{8 for $T_G=1$ \\ 4 for $T_G=2$ \\ 2 for $T_G=3$}\\
        RandAugment~\cite{randaugment}        &  	\checkmark  & 	\checkmark & 	\checkmark  & 	\checkmark \\
        Random erase~\cite{randerase}        &  	\xmark  & 	\checkmark & 	\checkmark  & 	\xmark \\
        \midrule
        \multicolumn{5}{l}{\hspace{-5pt}\textit{\textbf{Inference configuration}}} \\
        Testing views (temporal$\times$spatial)        &  	3 $\times$1  & 	1$\times$3 & 	2$\times$3  & 	1$\times$1 \\
        \bottomrule
        \end{tabular}\vspace{-5pt}
        % }
    \captionof{table}{Implementation details of \method.}\label{tab:imple_detail}
    \end{table*}
